# Supplementary material for: N-HiTS: Neural Hierarchical Interpolation for Time Series Forecasting
Source: arXiv:2201.12886 source file (2022-11-29)
Supplement: Supplementary file 1 [file concurrent.tex]

In the last year, interest in long-horizon forecasting applications caused a rapid growth of research dominated by Transformer-based forecasting methods. In addition to \Autoformer\ and \Informer, new variants, yet to be published, have been proposed, including \FEDformer, \ETSformer, \Preformer, \Triformer \citep{zhouFEDformer2022, wooETSformer2022, dazhaoPreformer2022, cirsteaTRIFormer2022}. 

For the completeness of our empirical evaluation, we include in Table~\ref{table:main_results_multivar_concurrent} the comparison with the concurrent research. Some caveats of this comparison are that these articles have not yet been peer-reviewed; some evaluations deviate in the length of the forecast horizons or don't report results for all the benchmark datasets, and finally, unfortunately, most studies only report a single run or don't report standard deviations in their accuracy measurements for which it is difficult to evaluate the significance of the results.

Table~\ref{table:main_results_multivar_concurrent} shows that \ours\ maintains MAE 11\% and MSE 9\% performance improvements across all the benchmark datasets and horizons. The only experiment setting where a concurrent research model outperforms \ours\ predictions is short-horizon \Exchange\ where \ETSformer\ reports MSE improvements of 9\% and MAE improvements of 4\%.

\begin{table*}[ht!]
% \tiny
\scriptsize
    \begin{center}
    \caption{Performance comparison with concurrent research, lower scores are better. Metrics for \ours\ are averaged over eight runs, best results are highlighted in bold.}
    \label{table:main_results_multivar_concurrent}    
	\begin{tabular}{ll | cccccccccc} \toprule
	&     & \multicolumn{2}{c}{\ours\ (Ours)}  & \multicolumn{2}{c}{FEDformer} & \multicolumn{2}{c}{ETSformer} & \multicolumn{2}{c}{Preformer} & \multicolumn{2}{c}{Triformer} \\
    &  Horizon & MSE        & MAE             & MSE            & MAE          & MSE             & MAE             & MSE        & MAE              & MSE         & MAE     \\ \midrule
\parbox[t]{0.2mm}{\multirow{4}{*}{\rotatebox[origin=c]{90}{\ETTm$_2$}}}
	& 96  & \textbf{0.176}  & \textbf{0.255}  & 0.203          & 0.287          & 0.183           & 0.275           & 0.213      & 0.295            & -           & -     \\
	& 192 & \textbf{0.245}  & \textbf{0.305}  & 0.269          & 0.328          & -               & -               & 0.269      & 0.329            & -           & -     \\
	& 336 & \textbf{0.295}  & \textbf{0.346}  & 0.325          & 0.366          & -               & -               & 0.324      & 0.363            & -           & -     \\
	& 720 & \textbf{0.401}  & 0.426           & 0.421          & 0.415          & -               & -               & 0.418      & \textbf{0.416}   & -           & -     \\ \midrule
\parbox[t]{0.2mm}{\multirow{4}{*}{\rotatebox[origin=c]{90}{$\quad$ \Electricity $\;$}}}
	& 96  & \textbf{0.147}  & \textbf{0.249}  & 0.183          & 0.297          & 0.187           & 0.302           & 0.180      & 0.297            & -           & -     \\
	& 192 & \textbf{0.167}  & \textbf{0.269}  & 0.195          & 0.308          & 0.196           & 0.311           & 0.189      & 0.302            & -           & -     \\
	& 336 & \textbf{0.186}  & \textbf{0.290}  & 0.212          & 0.313          & 0.215           & 0.330           & 0.201      & 0.319            & -           & -     \\
	& 720 & 0.243           & \textbf{0.340}  & \textbf{0.231} & 0.343          & 0.236           & 0.348           & 0.232      & 0.342            & -           & -     \\ \midrule
% \multirow{4}{0.1cm}{\Exchange}
\parbox[t]{0.2mm}{\multirow{4}{*}{\rotatebox[origin=c]{90}{\Exchange}}}
	& 96  & 0.092           & 0.211           & 0.139          & 0.276          & \textbf{0.083}  & \textbf{0.202}  & 0.148      & 0.282            & -           & -     \\
	& 192 & 0.208           & 0.322           & 0.256          & 0.369          & \textbf{0.180}  & \textbf{0.302}  & 0.268      & 0.378            & -           & -     \\
	& 336 & \textbf{0.341}  & \textbf{0.422}  & 0.426          & 0.464          & 0.354           & 0.433           & 0.447      & 0.499            & -           & -     \\
	& 720 & \textbf{0.888}  & \textbf{0.723}  & 1.090          & 0.800          & 0.996           & 0.761           & 1.092      & 0.812            & -           & -     \\ \midrule
% \multirow{4}{0.1cm}{\Traffic}
\parbox[t]{0.2mm}{\multirow{4}{*}{\rotatebox[origin=c]{90}{\TrafficL}}}        
	& 96  & \textbf{0.402}  & \textbf{0.282}  & 0.562          & 0.349          & 0.614           & 0.395           & 0.560      & 0.349            & -           & -     \\
	& 192 & \textbf{0.420}  & \textbf{0.297}  & 0.562          & 0.346          & 0.629           & 0.398           & 0.565      & 0.349            & -           & -     \\
	& 336 & \textbf{0.448}  & \textbf{0.313}  & 0.570          & 0.323          & 0.646           & 0.417           & 0.577      & 0.351            & -           & -     \\
	& 720 & \textbf{0.539}  & \textbf{0.353}  & 0.596          & 0.368          & 0.631           & 0.389           & 0.597      & 0.358            & -           & -     \\ \midrule
% \multirow{4}{0.1cm}{\Weather}
\parbox[t]{0.2mm}{\multirow{4}{*}{\rotatebox[origin=c]{90}{\Weather}}}        
	& 96  & \textbf{0.158}  & \textbf{0.195}  & 0.217          & 0.296          & 0.189           & 0.272           & 0.227      & 0.292            & -           & -     \\
	& 192 & \textbf{0.211}  & \textbf{0.247}  & 0.276          & 0.336          & 0.231           & 0.303           & 0.275      & 0.322            & -           & -     \\
	& 336 & \textbf{0.274}  & \textbf{0.300}  & 0.339          & 0.380          & 0.305           & 0.357           & 0.324      & 0.352            & -           & -     \\
	& 720 & \textbf{0.351}  & \textbf{0.353}  & 0.403          & 0.428          & 0.352           & 0.391           & 0.394      & 0.393            & -           & -     \\\midrule
% \multirow{4}{0.1cm}{\ILI}
\parbox[t]{0.2mm}{\multirow{4}{*}{\rotatebox[origin=c]{90}{\ILI}}}       
	& 24  & \textbf{1.862}  & \textbf{0.869}  & 2.203          & 0.963          & 2.862           & 1.128           & 3.143      & 1.185            & -           & -     \\
	& 36  & \textbf{2.071}  & \textbf{0.969}  & 2.272          & 0.976          & 2.683           & 1.029           & 2.793      & 1.054            & -           & -     \\
	& 48  & \textbf{2.184}  & 0.999           & 2.209          & \textbf{0.981} & 2.456           & 0.986           & 2.845      & 1.090            & -           & -     \\
	& 60  & \textbf{2.507}  & \textbf{1.060}  & 2.545          & 1.061          & 2.630           & 1.057           & 2.957      & 1.124            & -           & -     \\
    \bottomrule
	\end{tabular}
	\end{center}
\end{table*}

% We observed that on \Exchange\ accuracy measurements present high variance between each run, and most of the Transformer-based methods (including \ETSformer) do not report standard deviations on their accuracy measurements. As research progresses and the performance gap between models continues to shrink, it will be advisable to use statistical tests like Giacomini-White or Diebold-Mariano \citep{giacomini_white2006test, diebold_mariano1995test} to assess the performance differences significance. 
